# Supplementary material for: Bet and Attack: Incentive Compatible Collaborative Attacks Using Smart Contracts
Source: arXiv:2010.12280 source file (2021-09-23)
Supplement: Supplementary file 1 [file appendices.tex]

\begin{appendices}

%the following adds the word Appendix before the letter numbering
%\renewcommand{\thesection}{\appendixname~\Alph{section}}

\section{An appendix?}
\label{proofs}

\end{appendices}
